# Supplementary material for: Temperature dependence of magnetic anisotropy and domain wall tuning in BaTiO3(111)/CoFeB multiferroics
Source: arXiv:2305.07879 source file (2023-05-13)
Supplement: Supplementary file 1 [file BTO_111__T_dep_SI.pdf]

# Supplementary information for ‘Temperature Dependence of Magnetic Anisotropy and Domain Wall Tuning in $BaTiO_3$(111)/CoFeB Multiferroics’

R. G. Hunt,[1,2] K. J. A. Franke,[1] P. S. Keatley,[3] P. M. Shepley,[1,2] M. Rogers,[1,2] and T. A. Moore[1,2]

[1)] *School of Physics and Astronomy, University of Leeds, LS2 9JT, United Kingdom*

[2)] *Bragg Centre for Materials Research, University of Leeds, LS2 9JT, United Kingdom*

[3)] *Department of Physics and Astronomy, University of Exeter, Stocker Road, Exeter, EX4 4QL, United Kingdom*

## I. SUPPRESSION OF CHANGE IN MAGNETIC MOMENT ACROSS PHASE TRANSITIONS

We investigate the change in moment around the phase transition with respect to the applied field cooling/warming strength. This is shown in Fig. 1 in this supplementary material, where the measurement is repeated under increasing field strengths. Note that this sample is a repeat growth of the sample presented in the main paper, with a sample structure of BTO(111)/CoFeB(20nm)/Pt(5nm), but as the substrate is different the underlying ferroelectric domain structure is distinct from the sample used in the main paper. This leads to some difference in the transition behaviour which depends on the ferroelectric domain structure – notably, the tetragonal-orthorhombic transition initially leads to a decrease in moment.

Regardless, we find that an increasing field strength suppresses the overall magnitude of the change in the moment across the phase transitions and that for a magnetic field of 1000 mT the phase transitions do not significantly affect the magnitude of the moment. This, combined with the calculated Ms(T) behaviour shown in the main paper, leads us to conclude that there is no change in the saturation magnetization as a result of the strain.

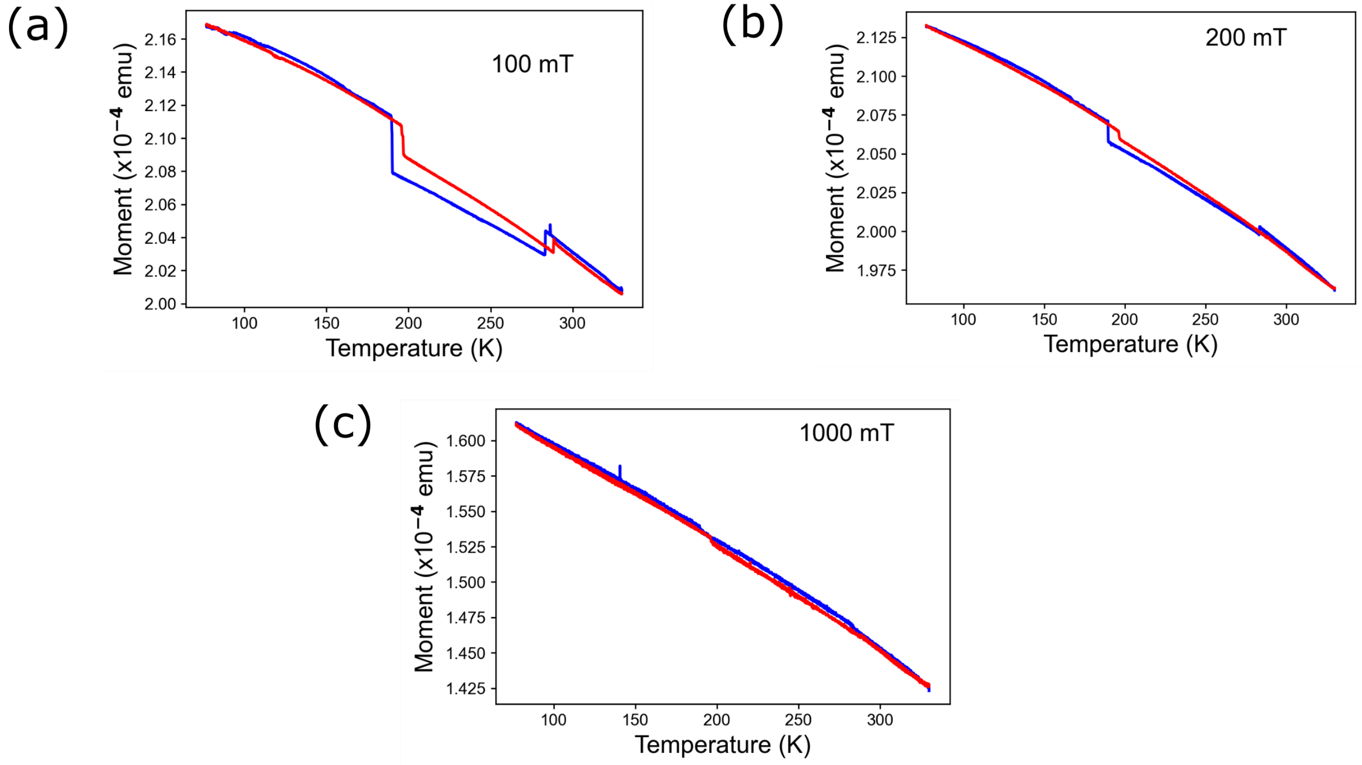


FIG. 1. Moment versus temperature measurements under a) 100 mT, b) 200 mT and c) 1000 mT applied magnetic fields. Blue lines indicate data taken while cooling, red lines indicate data taken while heating.

## II. CONFIGURATION OF MICROMAGNETIC SIMULATIONS

Here we will clarify the micromagnetic setup. As stated in the main text, the simulation is divided into three stripes of varying in-plane magnetoelastic anisotropy direction mimicking the ferroelectric domain structure. This is shown in Fig. 2a) for the case of a 60° rotation between the lattice elongations in the ferroelectric domains.

A magnetic field is then applied perpendicular to the domain wall (Fig. 2b) to initialize the uncharged magnetic domain wall state or parallel to the domain wall (Fig. 2c) to initialize the charged magnetic domain wall state. The magnetic field is then removed, and the system is relaxed to obtain the domain walls in Figs. 2b, c) under no applied magnetic field. Calculations of the domain wall width follow the equation laid out in the main paper,

$$\delta = \int_{-\infty}^{\infty} \cos^2(\phi')\, dx, \tag{1}$$

where $\phi$ is the angle of magnetization that varies with $x$. The bounds of the integral are in practice the centre of the stripe domains, which is always the furthest point from either of the two domain walls in the simulation space.

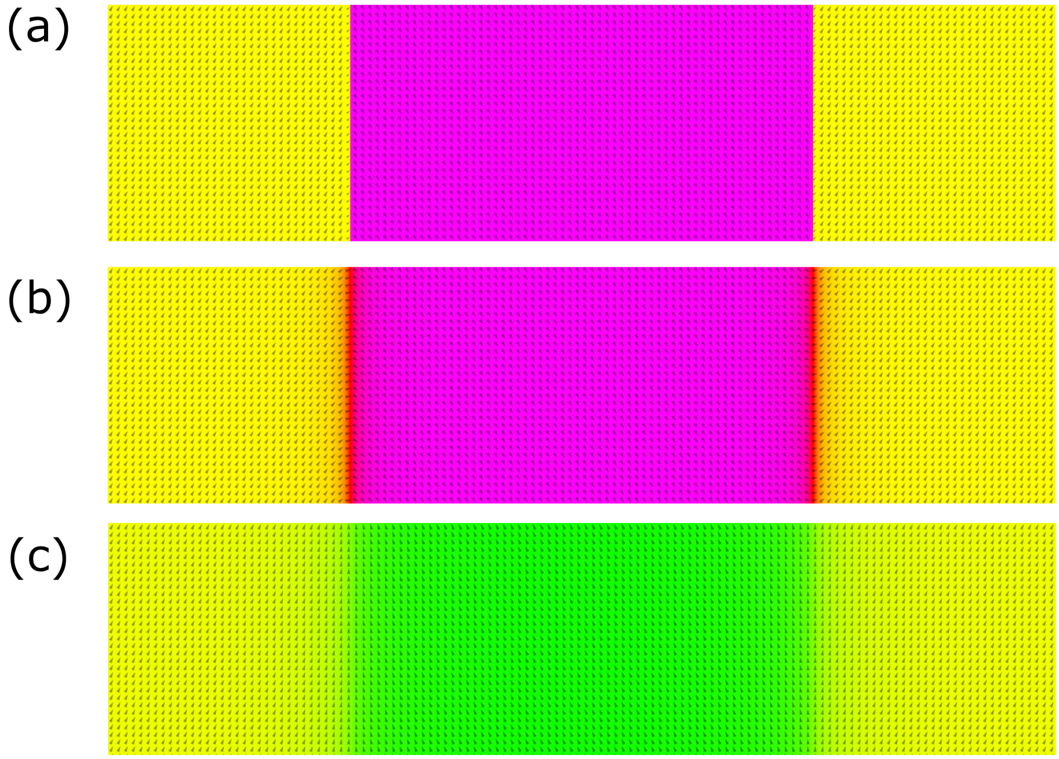


FIG. 2. Direction of in-plane magnetoelastic anisotropy within the micromagnetic simulations. b) Example of an uncharged magnetic domain wall configuration (60U). c) Example of a charged magnetic domain wall state (60C). Terminology is based on the main paper.
